# Supplementary material for: Boolean Abstractions for Realizability Modulo Theories (Extended version)
Source: arXiv:2310.17292 source file (2023-10-26)
Supplement: Supplementary file 1 [file 11-extendedPrelims.tex]

\section{Extended State of the Art} \label{appSec:stateOfArt}

\subsection{Preliminaries} \label{appSubSec:extendedPreliminaries}

%**THIS IS FULLY COPIED FROM SYNT.

We fix an alphabet $\Sigma$ and we call each element $a\in\alphabet$ a
{\em letter}.
In case of the Boolean version of the logic, $\AP$ is a set of {\em
  atomic propositions} and $\alphabet=2^\AP$ is the {\em alphabet}.
A {\em trace} is an infinite sequence $\sigma=a_0a_1\cdots$ of letters from 
$\alphabet$.
We denote the set of all infinite traces by $\alphabet^\omega$.
We use $\sigma(i)$ for $a_i$ and $\sigma^i$ for the suffix
$a_ia_{i+1}\cdots$.

\subsubsection{Linear Temporal Logic (LTL)}

Linear temporal logic (LTL) is a modal temporal logic with modalities
referring to time.
The syntax of LTL is the following:
\[
  \varphi  ::= T \DefOR a \DefOR \varphi \lor \varphi \DefOR \varphi \land \varphi \DefOR \neg \varphi
  \DefOR \Next \varphi \DefOR \varphi \U\varphi \DefOR \varphi \R\varphi
\]
where $a$ is an atomic proposition, $\lor$, $\land$ and $\neg$ are the
usual Boolean disjunction, conjunction and negation, and $\Next$, $\U$
and $\R$ are the next, until and release temporal operators.
The semantics of LTL associate traces $\sigma\in\Sigma^\omega$ with
formulae as follows:
 \[
   \begin{array}{l@{\hspace{0.3em}}c@{\hspace{0.3em}}l}
     \sigma \models T & \text{always} & \\
     \sigma \models a & \text{iff } & a \in\sigma(0) \\
     \sigma \models \varphi_1 \Or \varphi_2 & \text{iff } & \sigma\models \varphi_1 \text{ or } \sigma\models \varphi_2 \\
     \sigma \models \varphi_1 \And \varphi_2 & \text{iff } & \sigma\models \varphi_1 \text{ and } \sigma\models \varphi_2 \\
     \sigma \models \neg \varphi & \text{iff } & \sigma \not\models\varphi \\
     \sigma \models \Next \varphi & \text{iff } & \sigma^1\models \varphi \\
     \sigma \models \varphi_1 \U \varphi_2 & \text{iff } & \text{for some } i\geq 0\;\; \sigma^i\models \varphi_2, \text{ and } \\
                      & & \hspace{2em} \text{for all } 0\leq j<i, \sigma^j\models\varphi_1 \\
     \sigma \models \varphi_1 \R \varphi_2 & \text{iff } & \text{either for all } i\geq 0\;\; \sigma^i\models \varphi_2, \text{ or } \\
                      & & \hspace{1em} \text{for some } i\geq 0\;\; \sigma^i\models\varphi_1 \text{ and } \\
     & & \hspace{2em} \text{for all } 0\geq j\geq i\;\; \sigma^j\models\varphi_2 \\
   \end{array}
 \]
% \[
%   \begin{array}{l@{\hspace{0.5em}}l@{\hspace{0.5em}}l@{\hspace{3.8em}}l@{\hspace{0.3em}}c@{\hspace{0.3em}}l}
%     \sigma \models T & \text{always} & &
%     \sigma \models \varphi_1 \Or \varphi_2 & \text{iff } & \sigma\models \varphi_1 \text{ or } \sigma\models \varphi_2 \\
%     \sigma \models a & \text{iff } & \sigma(0)(a) = \True &
%     \sigma \models \neg \varphi & \text{iff } & \sigma \not\models\varphi \\
%     \sigma \models \Next \varphi & \text{iff } & \sigma^1\models \varphi &&& \\
%     \sigma \models \varphi_1 \U \varphi_2 & \text{iff } & \multicolumn{4}{l}{\text{for some } j\geq 0\;\; \sigma^j\models \varphi_2, \text{and for all } 0\leq i<j, \sigma^i\models\varphi_1}
%   \end{array}
% \]
%
 The set of temporal operators $\Next$, $\U$ and $\R$ is not minimal
 but admits a negation normal form.
 Common derived operators are $\Event\varphi\DefinedAs T \U\varphi$
 and $\Always\varphi\DefinedAs\Not\Event\Not\varphi$.
 A specification is called a safety specification if it only uses
 $\Next$ and $\Always$ in its negation normal form.

\subsubsection{Reactive synthesis and games}

Synthesis studies automatic generation of state machines from
high-level specifications.

Reactive synthesis
\cite{thomas08church,piteram06synthsis,bloem12synthesis,finkbeiner16synthesis,bloem21vacuity}
is the problem of producing a system from an LTL specification, where
the atomic propositions are split into propositions that are
controlled by the environment and those that are controlled by the
system.

%http://i-cav.org/cavlinks/wp-content/uploads/2019/07/ReactiveSynthesis_Lecture_1.pdf
Synthesis can be seen as a turn-based game, where in each turn the
environment produces values of its variables (inputs) and the
system responds with values of its variables (outputs).
A play is an infinite sequence of turns.
The system player wins a play according to an LTL formula $\varphi$ if
the trace of the play satisfies $\varphi$.
The arena of the game is the history of previous moves.
A strategy of a player is a map from the position into a move for the
player.
A play is played according to a strategy if all the moves of the
corresponding player are played according to the strategy.
A strategy is winning for a player if all the possible plays played
according to the strategy are winning.

In this paper we consider safety games, where the System wins if only
'safe' positions are visited (i.e. if the environment does not reach
an 'unsafe' position).

In this paper we consider the synthesis problem for theories, that is,
the set $\AP$ of atomic propositions is literals from some theory.
In this case, the alphabet is the possible valuations of the variables
(from the domains of the theories) and the atomic propositions
$a\in\AP$ are evaluated in the corresponding theories.
In terms of games, each player chooses in its turn a valuation of the
variables assigned to her.
We show in Section~\ref{sec:booleanAbs} a method that
reduces this problem to a purely Boolean synthesis problem.

\subsection{Reactivity Modulo Theories: Related work}

We call the \textit{reactivity modulo theory} to all those approaches that intend to add rich types (theory-based types) to the fields of LTL, reactive synthesis, infinite games and reactive systems overall.

There are many alternatives to LTL for specifying properties of
reactive systems, including
STL~\cite{ramanETAL2015reactiveSynthesisSignalTemporalLogic} and
GTL~\cite{cyrlukNarendran2001groundTemporalLogicHardwareVerification}.
We address here LTL with richer theories in the data, including a
large class of first-order theories, which have long been used in
verification
\cite{mannaPnueli1982verificationConcurrentProgramsTemporalProof}.

\subsubsection{Temporal stream logic}

Temporal Stream Logic (TSL) [1], was introduced as a new temporal logic for reactive synthesis that separates control from data. In the original TSL semantics, all functions and predicates are uninterpreted.

The difference with respect to our approach is that, because of the variable update operations TSL allows, its synthesis is undecidable in general, while we are exploring how to improve the limitations but keeping the synthesis problem decidable. In comparison, a limitation of our approach of course is that we cannot compare (rich) values across time which is an important aspect to explore in future work.

In addition, at [2], they extend TSL with first-order theories, enabling them to specify systems using interpreted functions and predicates such as incrementation or equality. They investigate the satisfiability problem of TSL modulo the theory of uninterpreted functions as well as with respect to Presburger arithmetic and the theory of equality: for all three theories, TSL satisfiability is also highly undecidable. Nevertheless, they identify three fragments of TSL for which the satisfiability problem is (semi-)decidable in the theory of uninterpreted functions and present an algorithm – which is not, obviously, guaranteed to terminate – for checking the satisfiability of a TSL formula in the theory of uninterpreted functions. This method scales well.

Also, at [3], they present a synthesis procedure for TSL(T), an extension of TSL with theories (arbitrary decidable theories in which quantifier elimination is possible). Synthesis is performed using a counter-example guided synthesis loop and an LTL synthesis procedure and. This part is similar to our extra requirement approach. Once again, they show that the synthesis problem for TSL(T) is undecidable, but propose a method that can successfully synthesize or show unrealizability of several non-Boolean examples.

\subsubsection{Other \textit{rich} temporal logics}

Another approach is Constraint LTL (CLTL)
\cite{demriDSouza2002automataTheoreticApproachConstraintLTL}, which extends
LTL with the possibility of expressing constraints between variables
at bounded distance (of time).
A constraint system $\mathcal{D}$ consists of a concrete domain and an
interpretation of relations on the domain. In Constraint LTL over
$\mathcal{D}$ (CLTL($\mathcal{D}$)), one can relate variables with
relations defined in $\mathcal{D}$. Similar to updates in TSL, CLTL
can specify assignment-like statements by utilizing the equality
relation. Like for all constraints allowing for a counting mechanism,
LTL with Presburger constraints, i.e.,
$\textit{CLTL}(\mathbb{Z}, =, +)$, is undecidable.
The difference with respect to our approach is that we do not allow
comparisons (in fact, no type of predicate) of variables within
different timesteps.

\subsubsection{Boolean abstraction-like ideas}

%from: https://dl.acm.org/doi/10.1007/978-3-030-38919-2_14#
In addition, variable automata with arithmetic enable the specification of reactive
systems with variables over an infinite domain of numeric values and
whose operation involves arithmetic manipulation
\cite{faranKupferman2018LTLArithmeticApplicationsReasoningHierarchical}
of these
values. \cite{faranKupferman2020synthesisSpecificationsArithmetic}
studies the synthesis problem for such specifications.

As for works closest to ours, the \cite{cheng2013numerical} preprint
proposes numerical LTL synthesis for cyber-physical systems, whose
calculations involve an interplay between an LTL synthesizer and a
nonlinear real arithmetic theory checker. However, their idea only
considers specifications where the arithmetic predicates belong to the
environment and indeed they \textit{overapproximate} the result.
Moreover, \cite{cheng2013numerical} does not contain full results.

Also, the problem of solving linear arithmetic games is addressed in
\cite{azadehKincaid2017strategySynthesisLinearArithmetic}, producing
algorithms for synthesizing winning strategies relying on a dedicated
decision procedure for quantified linear arithmetic formulae. However,
in addition to not being a Booleanization method, but a synthesis
method, they do not consider time modalities either.

\subsubsection{Infinite (state) games}

Since the specification that we will consider model infinite-state games, we also address this state of the art.

Many techniques, both explicit-state \cite{Thomas1995synthesisStrategiesInfiniteGames} and symbolic \cite{piterman06synthesis, hardingETAL2005newAlgorithmStrategySynthesisLTL}, are known for games on finite graphs.
%self
As for infinite-state games, a witness of a recent researches on them
is \cite{baier2021causalitybased} where a causality-based algorithm
for solving two-player reachability games represented by logical
constraints is presented, based on the notion of \textit{subgoals}.

%from: https://arxiv.org/pdf/2105.14247.pdf
Other approaches for solving infinite-state games include symbolic
BDD-based state-space exploration
\cite{edelkamp2002symbolicExplorationTwoPlayerGames}, computing
winning regions of both players using proof rules
\cite{beyeneETAL2014constraintApproachSolvingGamesInfinite} and
predicate abstraction
\cite{walkerRyzhyk2014predicateAbstractionReactiveSynthesis}. There is
also synthesis of infinite-state reactive implementations with random
behavior \cite{katis2020synthesisInfiniteRandom}.

\subsection{Reactivity modulo theories: Our domain} \label{appSubSec:arithmetics}

\subsubsection{Arithmetic first-order theories}

We use sorted first-order theories for extending the expressivity of
the atomic predicates.
For our purposes, a (sorted) first-order theory consists of (1) a
first-order vocabulary to form terms and predicates, (2) an
interpretation of the domains of the sorts, and (3) a reasoning system
to decide validity of sentences in the theory.

A particular class of first-order theories is that of arithmetic
theories, which are well studied in mathematics and theoretical
computer science, and are of particular relevance in formal
methods. Thus, even if the Boolean abstraction technique that we present allows any theory that is ddecidable on its $\exists^*\forall^*$ fragment, we are only considering arithmetic specifications in this paper, for illustrative reasons.

Note that all these theories are decidable.

We consider linear (arithmetic) theories:

\begin{itemize}
\item \textit{Linear Natural Arithmetic} or
  $\mathcal{T}_{\mathbb{N}}$ is the theory of natural numbers with
  addition but no arbitrary multiplication
  \cite{presburger1929theoremProving,davis1957presburgerImplementation,stansifer1984presburgersArticle,OPPEN1978upperBoundPresburger}. The
  signature is: $\Sigma_{\mathbb{N}} = \{ 0,1,\ldots,+,=\}$. One example of a
  literal is $(2x=4)$.
\item \textit{Linear Integer Arithmetic} or
  $\mathcal{T}_{\mathbb{Z}}$ the theory of integer numbers with
  addition but no arbitrary multiplication
  \cite{cooper1972theoremProving,Harrison2007IntroductionTL,zoharbradley2007Calculus,fischerRabin1998SuperExponentialComplexityPresburger}. The
  signature is
  $\Sigma_{\mathbb{Z}} = \{\ldots,-1,0,1,\ldots,,+,-,=,>\}$. A
  sentence literal is $(2x=-4)$.
    \item \textit{Linear Rational/Real Arithmetic} or
    $\mathcal{T}_{\mathbb{Q}}$: the theory of real/rational numbers with
    addition but no arbitrary multiplication
    \cite{Robinson1949DefinabilityAD,ferranteRackoff1975TheoryOfRationals,zoharbradley2007Calculus,Voigt2021Decidable}.
    The signature is $\Sigma_{\mathbb{Q}} = \{0,k,+,-,=,>\}$. For
    instance, a valid literal is $(2x=-\frac{1}{3})$.
\end{itemize}

And non-linear theories:

\begin{itemize}
    \item \textit{Nonlinear Real Arithmetic} or
    $\mathcal{T}_{\mathbb{R}}$ is the theory of real numbers with both
    addition and arbitrary multiplication
    \cite{tarski1951decisionElementary,seidenberg1954NewDecisionElementaryAlgebra,collins1975quantifierEliminationRealClosedCylindricalDecomposition,louVanDries1988alfredTarskiReal}.
    The signature is $\Sigma_{\mathbb{R}} = \{0,k,+,-,=,>,\cdot\}$.
    An example of a literal is $(2x^2=\frac{1}{3})$.
    \item Finally, we introduce \textit{Nonlinear Complex Arithmetic}
    or $\mathcal{T}_{\mathbb{C}}$, the theory of complex
    numbers with both addition and arbitrary multiplication
    \cite{ierardi1989quantifierEliminationAlgebraicallyClosed,ierardi1989ComplexityQuantifierEliminationAlgebraically,chistovGrigoriev2006complexityQuantifierEeliminationAlgebraically,harrison2008complexQuantifierHol}.
    The signature is $\Sigma_{\mathbb{C}} = \{0,k,+,-,=,>,\cdot, i\}$. For
    instance, a literal is $(2x^2=-3)$.
\end{itemize}

\subsubsection{Theory-augmented Linear Temporal Logic: \textit{LTL}$_\mathcal{T}$} \label{subSec:LTLt}

We extend LTL by accepting atomic propositions as literals from
theories.
We call $\textit{LTL}_{\mathcal{T}}$ to the extension of LTL where
there is a set of literals that are part of a first-order theory
$\mathcal{T}$.
In the realizability problem where theories are involved, the
variables that occur in the literals in the specification formula
$\varphi$ are split into those variables controlled by the environment
($\overline{v}_e$) and those controlled by the system
($\overline{v}_s$).
Thus, we have formulae $\varphi[\overline{v}_e, \overline{v}_s]$,
where $\overline{v}_e \cap \overline{v}_s = \emptyset$ and both if
$ v_e \in \overline{v}_e$ and $ v_s \in \overline{v}_s$, then
$v_e, v_s \in \mathcal{T}$.
Note that alphabet $\Sigma$ is now a valuation of the variables in
$\overline{v}_e$ and $\overline{v}_s$.
A trace is now an infinite sequence of valuations of the variables,
which induces an infinite sequence of Boolean values of the literals
that occurring in the specification, which in turn provide a valuation
of the formulae against the traces.

The realizability problem from an $\textit{LTL}_{\mathcal{T}}$
corresponds, in general, to a game with an infinite arena (and where
positions may have infinitely many successor if the ranges of the
variables controlled by the system and the environment are infinite).
For instance, consider an example formula from
$\textit{LTL}_{\mathbb{R}}$: $((x>1) \rightarrow \Next(y>x))$,
where $ x \in \overline{v}_e \wedge x: \mathbb{R}$ and
$ y \in \overline{v}_s \wedge y: \mathbb{R}$.
At time $0$, the environment may choose $\overline{v}_e^0=\{x^0=2\}$
environment valuation in timestep $0$, and the system may respond with
$\overline{v}_s^0=\{y^0=2\}$, with $\overline{v}_s^0=\{y^0=3\}$.
In this case, the choice $y^0=2$ makes the formula false so the
environment would win the play.

%As said, we are only considering arithmetic theories $\mathcal{T}_{\mathbb{N}}$, $\mathcal{T}_{\mathbb{Z}}$, $\mathcal{T}_{\mathbb{Q}}$, $\mathcal{T}_{\mathbb{R}}$, $\mathcal{T}_{\mathbb{C}}$ as $\mathcal{T}$.
