# Supplementary material for: Boolean Abstractions for Realizability Modulo Theories (Extended version)
Source: arXiv:2310.17292 source file (2023-10-26)
Supplement: Supplementary file 2 [file 7-supportMaterial.tex]

\section{Extra support material}

This section elaborates on the procedures presented (with algorithms) and the empirical evaluation (with tables). It is recommendable, yet not essential, to better understand the results.

\subsection{Algorithms in depth}

For the theoretical development (i.e., Section 3).

\begin{algorithm}
\SetAlgoLined
\textbf{Input: }$\phiT$\;
$\varphi'\gets \phiT[l_i \leftarrow s_i]$\;
$\calC \gets \textit{confs}(\textit{literals}(\phiT))$\;
$\calR \gets 2^{\calC}$\;
$\textit{VR} \gets \emptyset$\;
 \For{$(P,A) \in \calR$}{
   \If{$\exists\xs.\react_{(P,A)}(\xs)$ is valid}
   {
     $\textit{VR} \gets \textit{VR} \cup \{ (P,A) \}$\;
    }
 }
 $\displaystyle\phiExtra \gets \bigwedge_{(P,A)\in \textit{VR}} (e_{(P,A)} \rightarrow \bigvee_{c\in P} (\bigwedge_{l_i\in c}s_i\wedge \bigwedge_{l_i\notin c}\neg s_i))$ \;
 $\phiB \gets \varphi' \wedge \phiExtra$ \;
 \Return $\phiB$
 \caption{Brute-force Boolean Abstraction algorithm}
 \label{algoBruteForce}
\end{algorithm}

\begin{algorithm}[H] \label{algoModelLoop}
\SetAlgoLined
$\varphi'\gets \phiT[l_i \leftarrow s_i]$\;
 $\mathcal{C} \gets$ obtain\_the\_configutations\_from\_the\_literals\;
 $(\mathcal{P}, \mathcal{A}) \gets$ From $\mathcal{C}$, compute the sets of potentials and antipotentials \; 
 $\overline{c} \gets$ From  $\{\mathcal{C}, \mathcal{P}, \mathcal{A}\}$ obtain Boolean configurations, where $c \in \overline{c} \equiv p \in \mathcal{P}$ and $\neg c \in \overline{c} \equiv a \in \mathcal{A}$ \;
 Valid $\gets$ \{\}\;
 $\varphi = \exists \overline{c} \textit{. } \neg(\bigwedge_{0 \leq i \leq |\overline{c}|} \neg c_i) $\;
 \While{$\textit{SAT}(\varphi)$}{
    $m = model(\varphi)$\;
    $t = translate\_toTheory(m)$\; %\#For instance, from $c_0 \neg c_1 \neg c_2 c_3$ to \textit{PAAP}. 
    \If{$\exists \overline{x} :: (t)$ is valid}{
    $pos = take\_Positives(t)$ \;
    $\varphi = \varphi \wedge \neg(\bigwedge_{0 \leq j \leq |pos|} \neg pos_j)$ \;
    Valid $\gets$ Valid $\cup$ $(e_{\textit{t}}, pots(t))$\;
    %(i.e. Add: $fresh(\overline{e}) \implies Pots\_of(React_i)$) 
    }
    \Else{
    $neg = take\_Negatives(t)$ \;
    $\varphi = \varphi \wedge \neg(\bigwedge_{0 \leq k \leq |neg|} \neg neg_k)$ \;
    }
 }
 $\displaystyle\phiExtra \gets \bigwedge_{(P,A)\in \textit{VR}} (e_{(P,A)} \rightarrow \bigvee_{c\in P} (\bigwedge_{l_i\in c}s_i\wedge \bigwedge_{l_i\notin c}\neg s_i))$ \;
 %$\varphi^{extra} \gets get\_minimal(\varphi^{extra})$ \;
 $\phiB \gets \varphi' \wedge \phiExtra$ \;
 \Return $\varphi^{\mathbb{B}}$
 \caption{Model-loop based Boolean Abstraction algorithm}
\end{algorithm}

\begin{algorithm}[H] \label{algoDoubleSAT}
\SetAlgoLined
$\varphi'\gets \phiT[l_i \leftarrow s_i]$\;
 $\mathcal{C} \gets$ obtain\_the\_configutations\_from\_the\_literals\;
 $(\mathcal{P}, \mathcal{A}) \gets$ From $\mathcal{C}$, compute the sets of potentials and antipotentials \; 
 $\overline{c} \gets$ From  $\{\mathcal{C}, \mathcal{P}, \mathcal{A}\}$ obtain Boolean configurations, where $c \in \overline{c} \equiv p \in \mathcal{P}$ and $\neg c \in \overline{c} \equiv a \in \mathcal{A}$ \;
 Valid $\gets$ \{\}\;
 $\varphi = \exists \overline{c} \textit{. } \neg(\bigwedge_{0 \leq i \leq |\overline{c}|} \neg c_i) $\;
 \While{$\textit{SAT}(\varphi)$}{
    $m = model(\varphi)$\;
    $t = translate\_toTheory(m)$\; %\#For instance, from $c_0 \neg c_1 \neg c_2 c_3$ to \textit{PAAP}. 
    \If{$\exists \overline{x} :: (t)$ is valid}{
    $pos = take\_Positives(t)$ \;
    $\varphi = \varphi \wedge \neg(\bigwedge_{0 \leq j \leq |pos|} \neg pos_j)$ \;
    Valid $\gets$ Valid $\cup$ $(e_{\textit{t}}, pots(t))$\;
    %(i.e. Add: $fresh(\overline{e}) \implies Pots\_of(React_i)$) 
    }
    \Else{
    $neg = take\_Negatives(t)$ \;
    $\varphi = \varphi \wedge \neg(\bigwedge_{0 \leq k \leq |neg|} \neg neg_k)$ \;
    $also\_cut = inner\_loop (t)$ \; 
    \# We prune here all the space that the inner loop offers to cut.
    $\varphi = \varphi \wedge \neg(\bigwedge_{0 \leq w \leq |also\_cut|} \neg also\_cut_w)$ \;
    }
 }
 $\displaystyle\phiExtra \gets \bigwedge_{(P,A)\in \textit{VR}} (e_{(P,A)} \rightarrow \bigvee_{c\in P} (\bigwedge_{l_i\in c}s_i\wedge \bigwedge_{l_i\notin c}\neg s_i))$ \;
 %$\varphi^{extra} \gets get\_minimal(\varphi^{extra})$ \;
 $\phiB \gets \varphi' \wedge \phiExtra$ \;
 \Return $\varphi^{\mathbb{B}}$
 \caption{Double-SAT based Boolean Abstraction algorithm}
\end{algorithm}

\begin{algorithm}[H] \label{algoDefinitive}
\SetAlgoLined
 \textit{fatigue} \#This is the fixed number of inner-loops \;
 $division$ \#If the UNSAT outer model is divisible by this number, we enter the inner loop \;
 $\mathcal{S} \gets  get\_clusters(\textit{all\_literals})$ \;
 $\varphi^{extra} \gets \top$ \;
 \For{$s \in \mathcal{S}$}{
    $\varphi^{booleanized} \gets \{\}$ \;
    $\overline{l} \gets get\_literals(\mathcal{S})$ \#Cluster's literals \;
    \For {$0<r<|\overline{l}|$}{
     $\varphi^{booleanized} \gets \varphi^{booleanized} \cup \varphi^{Num}[l_r \leftarrow s_r]$ \;
    }
     $\mathcal{C} \gets$ obtain\_the\_configutations\_from\_the\_literals\;
     $(\mathcal{P}, \mathcal{A}) \gets$ From $\mathcal{C}$, compute the sets of potentials and antipotentials \; 
     $\overline{c} \gets$ From  $\{\mathcal{C}, \mathcal{P}, \mathcal{A}\}$ obtain Boolean configurations, where $c \in \overline{c} \equiv p \in \mathcal{P}$ and $\neg c \in \overline{c} \equiv a \in \mathcal{A}$ \;
     Valid $\gets$ \{\}\;
     $num\_unsats \gets 0$ \;
     $\varphi = \exists \overline{c} \textit{. } \neg(\bigwedge_{0 \leq i \leq |\overline{c}|} \neg c_i) $\;
     \While{$\textit{SAT}(\varphi)$}{
        $m = model(\varphi)$\;
        $t = translate\_toTheory(m)$\; %\#For instance, from $c_0 \neg c_1 \neg c_2 c_3$ to \textit{PAAP}. 
        \If{$\exists \overline{x} :: (t)$ is valid}{
        $pos = take\_Positives(t)$ \;
        $\varphi = \varphi \wedge \neg(\bigwedge_{0 \leq j \leq |pos|} \neg pos_j)$ \;
        Valid $\gets$ Valid $\cup$ $(e_{\textit{t}}, pots(t))$\;
        %(i.e. Add: $fresh(\overline{e}) \implies Pots\_of(React_i)$) 
        }
        \Else{
        $neg = take\_Negatives(t)$ \;
        $\varphi = \varphi \wedge \neg(\bigwedge_{0 \leq k \leq |neg|} \neg neg_k)$ \;
        
            \If{$num\_unsats \% division = 0$}{
                $also\_cut = inner\_loop (t, \textit{fatigue})$ \; 
                $\varphi = \varphi \wedge \neg(\bigwedge_{0 \leq w \leq |also\_cut|} \neg also\_cut_w)$ \
            }
        $num\_unsats = num\_unsats + 1$
        }
     }
 $\displaystyle\phiExtra \gets \bigwedge_{(P,A)\in \textit{VR}} (e_{(P,A)} \rightarrow \bigvee_{c\in P} (\bigwedge_{l_i\in c}s_i\wedge \bigwedge_{l_i\notin c}\neg s_i))$ \;
     %$\varphi^{extra}_s \gets get\_minimal(\varphi^{extra}_s)$ \;
     $\varphi^{extra} = \varphi^{extra} \wedge \varphi^{extra}_s$
    }

 $\phiB \gets \varphi' \wedge \phiExtra$ \;
 \Return $\varphi^{\mathbb{B}}$
 \caption{Definitive optimized Boolean Abstraction algorithm}
\end{algorithm}

\subsection{Tables}

For the empirical evaluation (i.e., Section 4).

\subsubsection{Synthetic tests}

We offer results of each test using its best heuristic-setup:

//SEVEN TABLES

\subsubsection{How we found the best heuristic-setups}

In order to discover the best heuristic-setups (at least for these datasets), we made a random search in a hyperparameter search-like idea:

In this paper, we offer a snapshot of it. Concretely, with test 0, we offer how we reached the best heuristic-setups for low cases (less than 5 literals), whereas with test N we show how we reached the best heuristic-setups for higher cases (greater than 4 literals).

//TWO TABLES

\subsubsection{Synthetic tests vs different theories}

We compare each test with the best heuristic-setup of previous section, against different theories.

Note that, in each test, one of the three theories corresponds to the original theory of the test, so each table is comparing the original theory against two modifications.

Test 0:

\begin{center} \label{tablTest0Theories}
\begin{tabular}{||c c c c||} 
 \hline
 Size version & $\mathcal{T}_{\mathbb{N}}$ & $\mathcal{T}_{\mathbb{Z}}$ & $\mathcal{T}_{\mathbb{R}}$ \\ 
 (literals) & (time) & (time) & (time) \\
  & (inner / outer) & (inner / outer) & (inner / outer) \\ [0.5ex] 
 \hline\hline
 2 & 30 & 60 & a\\ 
  & & 900 & a\\
 \hline
 3 & 30 & 16 & a \\
   &  & 30 & a \\
 \hline
 4 & 5 &  10 & a \\
 &  & 10 & a \\
 \hline
 5 & 3 &  4 & a \\
  &  & 3 & a \\
 \hline
 6 & 3 &  4 & a \\
  &  & 3 & a \\
 \hline
 7 & 3 &  4 & a \\
  & & 3 & a \\
 \hline
 8 & 3 &  4 & a \\
  & & 3 & a \\
 \hline
\end{tabular}
\end{center}

Test 1:

\begin{center} \label{tablTest0Theories}
\begin{tabular}{||c c c c||} 
 \hline
 Size version & $\mathcal{T}_{\mathbb{N}}$ & $\mathcal{T}_{\mathbb{Z}}$ & $\mathcal{T}_{\mathbb{R}}$ \\ 
 (literals) & (time) & (time) & (time) \\
  & (inner / outer) & (inner / outer) & (inner / outer) \\ [0.5ex] 
 \hline\hline
 2 & 30 & 60 & a\\ 
  & & 900 & a\\
 \hline
 3 & 30 & 16 & a \\
   &  & 30 & a \\
 \hline
 4 & 5 &  10 & a \\
 &  & 10 & a \\
 \hline
 5 & 3 &  4 & a \\
  &  & 3 & a \\
 \hline
 6 & 3 &  4 & a \\
  &  & 3 & a \\
 \hline
 7 & 3 &  4 & a \\
  & & 3 & a \\
 \hline
 8 & 3 &  4 & a \\
  & & 3 & a \\
 \hline
\end{tabular}
\end{center}

Test 2:

\begin{center} \label{tablTest0Theories}
\begin{tabular}{||c c c c||} 
 \hline
 Size version & $\mathcal{T}_{\mathbb{N}}$ & $\mathcal{T}_{\mathbb{Z}}$ & $\mathcal{T}_{\mathbb{R}}$ \\ 
 (literals) & (time) & (time) & (time) \\
  & (inner / outer) & (inner / outer) & (inner / outer) \\ [0.5ex] 
 \hline\hline
 2 & 30 & 60 & a\\ 
  & & 900 & a\\
 \hline
 3 & 30 & 16 & a \\
   &  & 30 & a \\
 \hline
 4 & 5 &  10 & a \\
 &  & 10 & a \\
 \hline
 5 & 3 &  4 & a \\
  &  & 3 & a \\
 \hline
 6 & 3 &  4 & a \\
  &  & 3 & a \\
 \hline
 7 & 3 &  4 & a \\
  & & 3 & a \\
 \hline
 8 & 3 &  4 & a \\
  & & 3 & a \\
 \hline
\end{tabular}
\end{center}

Test 3:

\begin{center} \label{tablTest0Theories}
\begin{tabular}{||c c c c||} 
 \hline
 Size version & $\mathcal{T}_{\mathbb{N}}$ & $\mathcal{T}_{\mathbb{Z}}$ & $\mathcal{T}_{\mathbb{R}}$ \\ 
 (literals) & (time) & (time) & (time) \\
  & (inner / outer) & (inner / outer) & (inner / outer) \\ [0.5ex] 
 \hline\hline
 2 & 30 & 60 & a\\ 
  & & 900 & a\\
 \hline
 3 & 30 & 16 & a \\
   &  & 30 & a \\
 \hline
 4 & 5 &  10 & a \\
 &  & 10 & a \\
 \hline
 5 & 3 &  4 & a \\
  &  & 3 & a \\
 \hline
 6 & 3 &  4 & a \\
  &  & 3 & a \\
 \hline
 7 & 3 &  4 & a \\
  & & 3 & a \\
 \hline
 8 & 3 &  4 & a \\
  & & 3 & a \\
 \hline
\end{tabular}
\end{center}

Test 4:

\begin{center} \label{tablTest0Theories}
\begin{tabular}{||c c c c||} 
 \hline
 Size version & $\mathcal{T}_{\mathbb{N}}$ & $\mathcal{T}_{\mathbb{Z}}$ & $\mathcal{T}_{\mathbb{R}}$ \\ 
 (literals) & (time) & (time) & (time) \\
  & (inner / outer) & (inner / outer) & (inner / outer) \\ [0.5ex] 
 \hline\hline
 2 & 30 & 60 & a\\ 
  & & 900 & a\\
 \hline
 3 & 30 & 16 & a \\
   &  & 30 & a \\
 \hline
 4 & 5 &  10 & a \\
 &  & 10 & a \\
 \hline
 5 & 3 &  4 & a \\
  &  & 3 & a \\
 \hline
 6 & 3 &  4 & a \\
  &  & 3 & a \\
 \hline
 7 & 3 &  4 & a \\
  & & 3 & a \\
 \hline
 8 & 3 &  4 & a \\
  & & 3 & a \\
 \hline
\end{tabular}
\end{center}

Test 5:

\begin{center} \label{tablTest0Theories}
\begin{tabular}{||c c c c||} 
 \hline
 Size version & $\mathcal{T}_{\mathbb{N}}$ & $\mathcal{T}_{\mathbb{Z}}$ & $\mathcal{T}_{\mathbb{R}}$ \\ 
 (literals) & (time) & (time) & (time) \\
  & (inner / outer) & (inner / outer) & (inner / outer) \\ [0.5ex] 
 \hline\hline
 2 & 30 & 60 & a\\ 
  & & 900 & a\\
 \hline
 3 & 30 & 16 & a \\
   &  & 30 & a \\
 \hline
 4 & 5 &  10 & a \\
 &  & 10 & a \\
 \hline
 5 & 3 &  4 & a \\
  &  & 3 & a \\
 \hline
 6 & 3 &  4 & a \\
  &  & 3 & a \\
 \hline
 7 & 3 &  4 & a \\
  & & 3 & a \\
 \hline
 8 & 3 &  4 & a \\
  & & 3 & a \\
 \hline
\end{tabular}
\end{center}

Test 6:

\begin{center} \label{tablTest0Theories}
\begin{tabular}{||c c c c||} 
 \hline
 Size version & $\mathcal{T}_{\mathbb{N}}$ & $\mathcal{T}_{\mathbb{Z}}$ & $\mathcal{T}_{\mathbb{R}}$ \\ 
 (literals) & (time) & (time) & (time) \\
  & (inner / outer) & (inner / outer) & (inner / outer) \\ [0.5ex] 
 \hline\hline
 2 & 30 & 60 & a\\ 
  & & 900 & a\\
 \hline
 3 & 30 & 16 & a \\
   &  & 30 & a \\
 \hline
 4 & 5 &  10 & a \\
 &  & 10 & a \\
 \hline
 5 & 3 &  4 & a \\
  &  & 3 & a \\
 \hline
 6 & 3 &  4 & a \\
  &  & 3 & a \\
 \hline
 7 & 3 &  4 & a \\
  & & 3 & a \\
 \hline
 8 & 3 &  4 & a \\
  & & 3 & a \\
 \hline
\end{tabular}
\end{center}

Test 7:

\begin{center} \label{tablTest0Theories}
\begin{tabular}{||c c c c||} 
 \hline
 Size version & $\mathcal{T}_{\mathbb{N}}$ & $\mathcal{T}_{\mathbb{Z}}$ & $\mathcal{T}_{\mathbb{R}}$ \\ 
 (literals) & (time) & (time) & (time) \\
  & (inner / outer) & (inner / outer) & (inner / outer) \\ [0.5ex] 
 \hline\hline
 2 & 30 & 60 & a\\ 
  & & 900 & a\\
 \hline
 3 & 30 & 16 & a \\
   &  & 30 & a \\
 \hline
 4 & 5 &  10 & a \\
 &  & 10 & a \\
 \hline
 5 & 3 &  4 & a \\
  &  & 3 & a \\
 \hline
 6 & 3 &  4 & a \\
  &  & 3 & a \\
 \hline
 7 & 3 &  4 & a \\
  & & 3 & a \\
 \hline
 8 & 3 &  4 & a \\
  & & 3 & a \\
 \hline
\end{tabular}
\end{center}

\subsubsection{Industrial tests}

We can see results cluster by cluster.

Case 1: Lift.

\begin{center} \label{tablLift}
\begin{tabular}{||c c c c c||} 
 \hline
 Cluster & Fix & Mod & Time & Quality \\ 
 (vars / lits) & (3 to 100) & (1,2,3 or 4) & (s) & (inner / outer) \\ [0.5ex] 
 \hline\hline
 $Cl_1$ & 30 & 2 & 32.38 &  60 \\ 
  (1, 7) &  &  & & 900 \\
 \hline
 $Cl_2$ & 30 & 2 & 1.27 &  16 \\
  (2, 4) &  &  & & 30 \\
 \hline
 $Cl_3$ & 5 & 2 & 0.57 &  10 \\
 (1, 3) &  &  & & 10 \\
 \hline
 $Cl_4$ & 3 & 2 & 0.23 &  4 \\
 (1, 2) &  &  & & 3 \\
 \hline
\end{tabular}
\end{center}

Case 2: Train

\begin{center} \label{tablTrain}
\begin{tabular}{||c c c c c||} 
 \hline
 Cluster & Fix & Mod & Time & Quality \\ 
 (vars / lits) & (3 to 100) & (1,2,3 or 4) & (s) & (inner / outer) \\ [0.5ex] 
 \hline\hline
 $Cl_1$ & 30 & 2 & 2.33 &  26 \\ 
 (1, 3) &  &  & & 60 \\
 \hline
 $Cl_2$ & 30 & 2 & 0.11 &  2 \\
  (2, 1) &  &  & & 0 \\
 \hline
 $Cl_3$  & 30 & 2 & 0.29 &  2 \\
 (1, 3) &  &  & & 13 \\
 \hline
 $Cl_4$ & 30 & 2 & 0.23 &  3 \\
 (1, 1) &  &  & & 2 \\
 \hline
 $Cl_{5.1}$ & 30 & 2 & 833.32 &  1620 \\
 (3, 6) &  &  & & 9199 \\
 \hline
 $Cl_{5.2}$ & 30 & 2 & EXEC &  EXEC \\
 (4, 6) &  &  & & EXEC \\
 \hline
 $Cl_{6.1}$ & 30 & 2 & EXEC &  EXEC \\
 (2, 4)  &  &  & & EXEC \\
 \hline
 $Cl_{6.2}$ & 30 & 2 & 6571.9738 &  2728 \\
 (3, 12) &  &  & & 40920 \\
 \hline
\end{tabular}
\end{center}

Case 3: Connect

\begin{center} \label{tablConnect}
\begin{tabular}{||c c c c c||} 
 \hline
 Cluster & Fix & Mod & Time & Quality \\ 
 (vars / lits) & (3 to 100) & (1,2,3 or 4) & (s) & (inner / outer) \\ [0.5ex] 
 \hline\hline
 $Cl_{\textit{unique}}$ & 30 & 2 & 0.12 &  4 \\ 
  (2, 2) &  &  & & 0 \\
 \hline
\end{tabular}
\end{center}

Case 4: Cooker

\begin{center} \label{tablCooker}
\begin{tabular}{||c c c c c||} 
 \hline
 Cluster & Fix & Mod & Time & Quality \\ 
 (vars / lits) & (3 to 100) & (1,2,3 or 4) & (s) & (inner / outer) \\ [0.5ex] 
 \hline\hline
 $Cl_{\textit{unique}}$ & 30 & 2 & 2.82 &  8 \\ 
  (3, 5) &  &  & & 120 \\
 \hline
\end{tabular}
\end{center}

Cooker has been a good showing of how different SAT-paths yield totally different performances: there have been other paths: from 7 seconds with (18+270) to 200 seconds with (3853+270), all of them with the same heuristic-setup.

Case 5: (Two) Tanks

//The most complex one

Case 6: Usb

\begin{center} \label{tablUSB}
\begin{tabular}{||c c c c c||} 
 \hline
 Cluster & Fix & Mod & Time & Quality \\ 
 (vars / lits) & (3 to 100) & (1,2,3 or 4) & (s) & (inner / outer) \\ [0.5ex] 
 \hline\hline
 $Cl_{\textit{unique}}$ & 30 & 2 & 0.26 &  8 \\ 
  (2, 3) &  &  & & 0 \\
 \hline
\end{tabular}
\end{center}

Also tested a (synthetic) modification with (3, 5), in 1390.75 seconds and (18038+0) queries.

Case 7: Stages

\begin{center} \label{tablStages}
\begin{tabular}{||c c c c c||} 
 \hline
 Cluster & Fix & Mod & Time & Quality \\ 
 (vars / lits) & (3 to 100) & (1,2,3 or 4) & (s) & (inner / outer) \\ [0.5ex] 
 \hline\hline
 $Cl_A$ & 30 & 2 & 34.25 &  256 \\ 
 (8, 8) &  &  & & 0 \\
 \hline
 $Cl_B$ & 30 & 2 & 2895.74 &  25216 \\
 (8, 11) &  &  & & 2790 \\
 \hline
\end{tabular}
\end{center}

Note that Booleanization has worked so well that they have even wrapped real clusters 1 and 2 into cluster A and wrapped real clusters 3 and 4 into cluster B. This is an example of how a simple coupling (in this case, a single player) yields a simpler Boolean abstractions (and, potentially, a simple synthesis).

\subsubsection{Percentages of coverage}

Here we show the most interesting percentages of coverage in each literal amount, from 2 to 12. Concretely, we show the number of outer+inner queries compared to the total number of queries that would be necessary in an exhaustive-like algorithm. We also show which test yields each result.

\begin{itemize}
    \item $2$ literals, $106.666$\% of queries. Concretely: 
    \begin{itemize}
        \item ($4+14$) out of 15.
    \end{itemize}
    \item 3 literals, 44.705\% of queries:
    \begin{itemize}
        \item ($10+104$) out of 255.
    \end{itemize}
    \item 4 literals, 0.70649271381704\% of queries. Concretely: 
    \begin{itemize}
        \item ($83+380$) out of 65535.
    \end{itemize}
    \item 5 literals, 0.00007203780116\% of queries. Concretely: 
    \begin{itemize}
        \item ($334+2760$) out of 4294967295.
    \end{itemize}
    \item 6 literals, 0.0000000000001222\% of queries. Concretely: 
    \begin{itemize}
        \item ($2074+20470$) out of 18446744073709551615.
    \end{itemize}
    \item 7 literals, 0.00000000000000000000000000000003947\% of queries. Concretely: 
    \begin{itemize}
        \item ($8363+125940$) out of 340282366920938463463374607431768211455.
    \end{itemize}
    ...
    \item 12 literals,which hugely tends to 0\% of queries. Concretely: 
    \begin{itemize}
       \item ($2728+40920$) out of \\
    1797693134862315907729305190789024733617976978942306572734300811577326758055... \\ ...0096313270847732240753602112011387987139335765878976881441662249284743063947... \\ ...4124377767893424865485276302219601246094119453082952085005768838150682342462... \\ ...881473913110540827237163350510684586298239947245938479716304835356329624224137215
    \end{itemize}
\end{itemize}

Note that we are mixing both synthetic and industrial (the biggest ones) examples in these examples.
