# Supplementary material for: Boolean Abstractions for Realizability Modulo Theories (Extended version)
Source: arXiv:2310.17292 source file (2023-10-26)
Supplement: Supplementary file 3 [file 8-extraOptimizations.tex]

\section{Extra optimizations} \label{appSec:optimizations}

%We choose some basic heuristics that are combined. They are depicted in Alg.~\ref{algoDefinitive}.

\subsubsection{Main Antipotential core}

This heuristic consists of the following: once an outer model is obtained, it is asked whether the combination of all the antipotentials in conjunction is $\top$ or not (this is called the \textit{Main Antipotential Core}). If the Main core is $\perp$, then it is very likely that there exists an $\perp$ core that is a subcombination of the main one. On the other hand, if the main core is $\top$, then we already know (by logical argument) that we will not find $\perp$ cores purely composed of antipotentials, so the search for the inner loop is likely to be fruitless. Therefore, we enter the inner loop if and only if that Main core is $\perp$. 

For instance, let an outer loop model be $\textit{PAPA}$. If we query $\textit{?A?A}$ and we obtain $\perp$, then probably some subcombination (e.g., $\textit{???A}$) will be $\perp$, thus be an $\perp$ core. Else, if we obtained $\top$, then all the subcombinations will be $\top$, so there is no point in searching deeper.

We saw that using this heuristic, from a few outer models where the inner loop has been entered, in the following outer models the inner loops are hardly entered. The result is that the number of inner and outer models is balanced, producing much better times and number of queries.

%Note that the following two heuristics (and any other that is not explicitly mentioned) incorporate this heuristic, regardless of their internal parameters.

\subsubsection{Naive heuristics}

We have also proposed three very simple heuristics in order to balance the number of turns of the outer and inner loops; forcing, in particular, that there are more models in the outer loop

First, we have the fixed number of inner loops, which, as its name suggests, simply sets the maximum number of models that the inner loop can explore before cutting it and going to the next outer model. This idea is especially effective in (1) requirements with many literals, because the tree is larger to explore; and (2) the more outer models that have been already output, because more $\top$ results are likely to appear and thus explored in vain.

The second idea is that a division by module decides whether or not to enter the inner loop. Specifically, there is a counter for the number of times an $\perp$ model has been explored from the outer to the inner loop; the idea, then, is that when that number is divisible by another number that is chosen, only then the inner loop is entered. In this way, for example, only the $\perp$ that have come out in an even position are scanned.

The third idea is adding a decay over the quantity of times that we enter the inner loop. The reason fort this is that, (1) at the very beginning we extract a lot of information from each inner-loop, whereas (2) whenever the exploration moves forward, we get less information from it. Thus, we are interested in limiting the fuel used in inner loops, so we do it using a decay function. We implemented intuitive versions of this function, such as decreasing the fatigue in 1 unit for each 40 enters in inner-loops. Decays can also be discrete or continuous, but this is out of th escope of this paper.

\subsubsection{Preprocessing: Clustering}

This is a useful technique for reducing the size of the problem in a pre-processing-like phase.

To \textit{clusterize} the original requirements means making \textit{islands} of literals that share variables. If two islands do not share any variable, we can perform Boolean abstraction to them separatedly.

The algorithm for performing clustering is straightforward. All variables are traversed: for each (say $a$), its neighbours are stored; for the next variable (say $b$), if $a$ is a neighbour, then $b$ attaches not only the $a$ as a neighbour, but also all the neighbours of $a$. Thus, at the end we obtain $n \leq numVariable$ clusters that can be separatedly Booleanized.

For instance, given $\varphi = \square (((a>b) \implies (b>c)) \wedge ((e>f) \implies (d>g)) \wedge ((c>t) \implies (g>v))$, the algorithm Booleanized $(a>b) \implies (b>c))$ and $((c>t) \implies (g>v))$ on one process (since $c$ \textit{links} both clusters), and $((e>f) \implies (d>g))$ in another process. Then, both generated extra requirements are conjuncted.
