# Supplementary material for: Boolean Abstractions for Realizability Modulo Theories (Extended version)
Source: arXiv:2310.17292 source file (2023-10-26)
Supplement: Supplementary file 4 [file 8-futureWork.tex]

\section{Future work} \label{appSec:futureWork}

In this paper, we showed that if variables do not
relate over time then $\LTLt$ realizabilty is decidable (for $\exists^*\forall^*$-
decidable theories theories); however, it is easy to see that if one can relate variables
arbitrarily, we can build two counter machines (or TSL) to \textit{Super}$\LTLt$-realizability 
(proving undecidability). Thus, we are studying controlled (and useful) ways 
to pass information between temporal states; i.e., restricted forms of predicates
that relate variables accross time. This allows us to enrich TSL so that benchmarks that previously
were semi-decidable and hard to solve (e.g., experiment $5$ in \cite{maderbacherBloem2021reactiveSynthesisModuloTheoriesAbstraction}) 
become decidable and easily solvable expressed in $\LTLt$ and translated with Boolean Abstraction.
  
As for other ongoing challenges, they focus on the followings:

\begin{itemize}
    \item Enhancing the scalibility of the Boolean abstraction algorithm.
    Some of these optimizations rely on theory-based reasoning, whereas others
    exploit well-known decision procedures such as Cooper's quantifier
    elimination method~\cite{cooper1972theoremProving}.
    \item Expanding the expressive fragment of Boolean abstraction while maintaining decidability. 
    We are studiying its usage with non-arithmetic theories such as the 
    \textit{Theory of Arrays}~\cite{bradleyETAL2006whatDecidableAboutArrays}.
  \item Extending applicability of Boolean abstraction in different
    contexts.  For instance, Boolean abstraction can be used to
    pre-check the realizability of (rich) specifications to be used in monitors of runtime
    verification~\cite{gorostiagaSanchez2022hlolaVeryFunctionalStreamRV}.
\end{itemize}

Also, we are researching how to move from realizability modulo theories, to
(reactive) synthesis modulo theories, on realizable instances. The missing piece is 
the function that provides the system's values given environment's values that make 
the corresponding (Boolean) literals true. This function is guaranteed to exist, but 
we need to realize it as a computable function in some programming language.
Our early results are promising, and they suggest that this function can be obtained using an interplay 
between the algorithm that produces the extra formula and existential queries in SMT solvers.
However, we suspect there are ways to obtain more lightweight systems.

Note that Appendix~\ref{appSec:moreEmpirical} also contains interesting issues and work in progress
about empirical evaluation.
