# Supplementary material for: Boolean Abstractions for Realizability Modulo Theories (Extended version)
Source: arXiv:2310.17292 source file (2023-10-26)
Supplement: Supplementary file 5 [file 9-newBenchmarking.tex]

\section{Benchmarks in depth}

\subsection{Foundations}

We make use of other seven real industrial specifications in order to test the Boolean abstraction against problems of the industry; which also allows us to see patterns that recur when designing optimizations. These are these specification’s names \footnote{Note that we keep their names at minimum, and they have been altered in order not to reveal true industrial information. Also, note that they belong to different production areas whose particular usages are out of the scope of this article.}:

\begin{itemize}
    \item \textit{Lift}: This specification is part of a set of specifications that describes the functioning of a freight elevator system (see Appendix T1). It is composed of N requirements, it contains X literals and Y variables.
    \item \textit{Train}: This specification is part of a set of specifications describing the functioning of an autonomous train driving system (see Appendix T2). It is composed of N requirements, it contains X literals and Y variables.
    \item \textit{Connect}: This specification is part of a set of specifications describing the functioning of an electric vehicle charging and discharging system (see Appendix T3). It is composed of N requirements, it contains X literals and Y variables.
    \item \textit{Cooker}: This specification is part of a set of specifications describing the functioning of a system consisting of two independently operating liquid pumping tanks (see Appendix T4). It is composed of N requirements, it contains X literals and Y variables.
    \item \textit{Tanks}: This specification is part of a set of specifications describing the operation of a food processor with various functions (see Appendix T5). It is composed of N requirements, it contains X literals and Y variables.
    \item \textit{Usb}: This specification is part of a set of specifications describing the operation of a system that prevents the loss of information during the interaction between a USB and a machine (see Appendix T6). It is composed of N requirements, it contains X literals and Y variables.
    \item \textit{Stage}: This specification is part of a set of specifications describing the operation of a system that combines the use of different sensors for use in aviation (see Appendix T7). It is composed of N requirements, it contains X literals and Y variables.
\end{itemize}

Industrial specifications' literals can be found, as well as its clusters. Note that, as for industrial specifications.  the original ones belong to an enterprise \footnote{The company is: \url{https://www.developair.tech}} and, thus:

\begin{itemize}
    \item We add a short natural language description of what type of system has been requested (e.g., "this is a specification describing how a train behaves").
    \item We use only the literals we are interested in, i.e., the numerical ones, ignoring the original specification, temporality, Boolean variables etc (e.g., "$lit_1 = (x< 1000), lit_2 = (y >= z+1)$").
    \item We change the variable names, so that nothing is really intuited about the original specification (e.g., from '\textit{transistor\_voltage}' to '\textit{p}').
\end{itemize}

\subsubsection{Test by test}

\subsubsection{Industrial case 1: Lift}

This specification is part of a set of specifications that describes the functioning of a freight elevator system.

Concretely, different floors are selected on which to stop based on different weight parameters.

The full specification can be found in Appendix N, whereas the arithmetic/enumerated specification is the following:

//It is divided in clusters 1...

//As for cluster 1...

\subsubsection{Industrial case 2: Train}

This specification is part of a set of specifications describing the functioning of an autonomous train driving system.

Concretely, different sensors are read to know whether or not the doors can be closed after stopping at a station.

The full specification can be found in Appendix N, whereas the arithmetic/enumerated specification is the following:

//

\subsubsection{Industrial case 3: Connect}

This specification is part of a set of specifications describing the functioning of an electric vehicle charging and discharging system.

Concretely, different readings are obtained on the voltages of the load points to decide how to level the input and output power flow.

The full specification can be found in Appendix N, whereas the arithmetic/enumerated specification is the following:

//

\subsubsection{Industrial case 4: Two tanks}

This specification is part of a set of specifications describing the functioning of a system consisting of two independently operating liquid pumping tanks.

Concretely, it fluctuates between different heights in tank capacities, based on sensor readings of liquid flow rates.

The full specification can be found in Appendix N, whereas the arithmetic/enumerated specification is the following:

//

\subsubsection{Industrial case 5: Cooker}

This specification is part of a set of specifications describing the operation of a food processor with various functions.

Concretely, using internal information about the time and external information about the user, it varies between different cooking modes and intensities.

The full specification can be found in Appendix N, whereas the arithmetic/enumerated specification is the following:

//

\subsubsection{Industrial case 6: Usb}

This specification is part of a set of specifications describing the operation of a system that prevents the loss of information during the interaction between a USB and a machine.

Concretely, it features different security modes, as well as error handling and different possible connections between the USB and the machine.

The full specification can be found in Appendix N, whereas the arithmetic/enumerated specification is the following:

//

\subsubsection{Industrial case 7: Stages}

This specification is part of a set of specifications describing the operation of a system that combines the use of different sensors for use in aviation.

Concretely, it is shown how the readings of a pitot tube are managed, based on some resistor's temperatures, power voltages and tubes' altitude lectures.

The full specification can be found in Appendix N, whereas the arithmetic/enumerated specification is the following:

//
