# Supplementary material for: Boolean Abstractions for Realizability Modulo Theories (Extended version)
Source: arXiv:2310.17292 source file (2023-10-26)
Supplement: Supplementary file 6 [file 13-semanticsLTL.tex]

\section{Semantics of LTL}

The semantics of LTL associate traces $\sigma\in\Sigma^\omega$ with
formulae as follows:
 \[
   \begin{array}{l@{\hspace{0.3em}}c@{\hspace{0.3em}}l}
     \sigma \models T & \text{always} & \\
     \sigma \models a & \text{iff } & a \in\sigma(0) \\
     \sigma \models \varphi_1 \Or \varphi_2 & \text{iff } & \sigma\models \varphi_1 \text{ or } \sigma\models \varphi_2 \\
     \sigma \models \varphi_1 \And \varphi_2 & \text{iff } & \sigma\models \varphi_1 \text{ and } \sigma\models \varphi_2 \\
     \sigma \models \neg \varphi & \text{iff } & \sigma \not\models\varphi \\
     \sigma \models \Next \varphi & \text{iff } & \sigma^1\models \varphi \\
     \sigma \models \varphi_1 \U \varphi_2 & \text{iff } & \text{for some } i\geq 0\;\; \sigma^i\models \varphi_2, \text{ and } \\
                      & & \hspace{2em} \text{for all } 0\leq j<i, \sigma^j\models\varphi_1 \\
     \sigma \models \varphi_1 \R \varphi_2 & \text{iff } & \text{either for all } i\geq 0\;\; \sigma^i\models \varphi_2, \text{ or } \\
                      & & \hspace{1em} \text{for some } i\geq 0\;\; \sigma^i\models\varphi_1 \text{ and } \\
     & & \hspace{2em} \text{for all } 0\geq j\geq i\;\; \sigma^j\models\varphi_2 \\
   \end{array}
 \]
 The set of temporal operators $\Next$, $\U$ and $\R$ is not minimal
 but admits a negation normal form.
 Common derived operators are $\Event\varphi\DefinedAs T \U\varphi$
 and $\Always\varphi\DefinedAs\Not\Event\Not\varphi$.
 A specification is called a safety specification if it only uses
 $\Next$ and $\Always$ in its negation normal form.
 In this paper we consider standard (future) LTL, and no variation of this one, such as Past LTL~\cite{Gabbay1980OnTT}.
