# Supplementary material for: Boolean Abstractions for Realizability Modulo Theories (Extended version)
Source: arXiv:2310.17292 source file (2023-10-26)
Supplement: Supplementary file 8 [file 8-algorithmsDepth.tex]

\section{Algorithms unrolled}

Note the \textit{for} loop in the Alg~\ref{algoBruteForce} and the \textit{while} loop in Alg~\ref{algoModelLoop}.

Note the heuristics in Alg. \ref{algoDefinitive}.

\begin{algorithm}[H] \label{algoDefinitive}
\SetAlgoLined
\textbf{Input: }$\phiT$\;
 \textit{fatigue}, \textit{division} \#These are (1) the fixed number of inner-loops and (2) if UNSAT outer model is divisible by this number, we enter inner-loop \;
 $\mathcal{S} \gets  get\_clusters(\textit{all\_literals})$ \;
 $\varphi^{extra} \gets \top$ \;
 \For{$s \in \mathcal{S}$}{
    $\varphi^{''} \gets \{\}$ \;
    $\overline{l} \gets get\_literals(\mathcal{S})$ \#Cluster's literals \;
    \For {$0<r<|\overline{l}|$}{
     $\varphi^{''} \gets \varphi^{''} \cup \varphi^{Num}[l_r \leftarrow s_r]$ \;
    }
     $\mathcal{C} \gets$ obtain\_the\_configutations\_from\_the\_literals\;
     $(\mathcal{P}, \mathcal{A}) \gets$ From $\mathcal{C}$, compute the sets of potentials and antipotentials \; 
     $\overline{c} \gets$ From  $\{\mathcal{C}, \mathcal{P}, \mathcal{A}\}$ obtain Boolean configurations, where $c \in \overline{c} \equiv p \in \mathcal{P}$ and $\neg c \in \overline{c} \equiv a \in \mathcal{A}$ \;
     Valid $\gets$ \{\}\;
     $num\_unsats \gets 0$ \;
     $\varphi = \exists \overline{c} \textit{. } \neg(\bigwedge_{0 \leq i \leq |\overline{c}|} \neg c_i) $\;
     \While{$\textit{SAT}(\varphi)$}{
        $t = translate\_toTheory(model(\varphi))$\;
        %$t = translate\_toTheory(m)$\; %\#For instance, from $c_0 \neg c_1 \neg c_2 c_3$ to \textit{PAAP}. 
        \If{$\exists \overline{x} :: (t)$ is valid}{
        $pos = take\_Positives(t)$ \;
        $\varphi = \varphi \wedge \neg(\bigwedge_{0 \leq j \leq |pos|} \neg pos_j)$ \;
        Valid $\gets$ Valid $\cup$ $(e_{\textit{t}}, pots(t))$\;
        %(i.e. Add: $fresh(\overline{e}) \implies Pots\_of(React_i)$) 
        }
        \Else{
        $neg = take\_Negatives(t)$ \;
        $\varphi = \varphi \wedge \neg(\bigwedge_{0 \leq k \leq |neg|} \neg neg_k)$ \;
        
            \If{$num\_unsats \% division = 0$}{
                $also\_cut = inner\_loop (t, \textit{fatigue})$ \; 
                $\varphi = \varphi \wedge \neg(\bigwedge_{0 \leq w \leq |also\_cut|} \neg also\_cut_w)$ \;
            }
        $num\_unsats = num\_unsats + 1$
        }
     }
 $\displaystyle \varphi^{extra}_s \gets \bigwedge_{(P,A)\in \textit{VR}} (e_{(P,A)} \rightarrow \bigvee_{c\in P} (\bigwedge_{l_i\in c}s_i\wedge \bigwedge_{l_i\notin c}\neg s_i))$ \;
     %$\varphi^{extra}_s \gets get\_minimal(\varphi^{extra}_s)$ \;
     $\varphi^{extra} = \varphi^{extra} \wedge \varphi^{extra}_s$
    }

 $\phiB \gets \varphi' \wedge \phiExtra$ \;
 \Return $\varphi^{\mathbb{B}}$
 \caption{Double SAT algorithm with heuristics}
\end{algorithm}
